# Supplementary material for: On birational automorphisms of double EPW-cubes
Source: arXiv:2405.15510 ancillary file (2024-12-27)
Supplement: Supplementary file 1 [file tablefull-3.pdf]

| Leech id | $G$             | $(\#(-12, 2), \#(-36, 2))$ | $\mathbf{L}_{\mathbf{K3}[3]}^G$                                                                                                                                                                       | $D$      |
|----------|-----------------|----------------------------|-------------------------------------------------------------------------------------------------------------------------------------------------------------------------------------------------------|----------|
| 1        | $C_1$           | $(0, 0)$                   | $\mathbf{L}_{\mathbf{K3}[3]}$                                                                                                                                                                         | $\times$ |
| 2        | $C_2$           | $(0, 0)$                   | $U^{\oplus 3} \oplus E_8(-2) \oplus [-4]$                                                                                                                                                             | $\times$ |
| 3        | $C_2^2$         | $(0, 0)$                   | $U \oplus U(2)^{\oplus 2} \oplus D_4(-2) \oplus [-4]$                                                                                                                                                 | $\times$ |
|          |                 | $(64, 0)$                  | $U^{\oplus 2} \oplus U(2) \oplus D_4(-2) \oplus [-4]$                                                                                                                                                 | $\times$ |
| 4        | $C_3$           | $(0, 0)$                   | $U^{\oplus 2} \oplus U(3) \oplus A_3(-3) \oplus A_2(-1)$                                                                                                                                              | $\times$ |
| 5        | $C_2$           | $(32, 0)$                  | $U(2)^{\oplus 2} \oplus [-2]^{\oplus 4} \oplus [-4] \oplus \begin{pmatrix} 0 & 2 \\ 2 & -2 \end{pmatrix}$                                                                                             | $\times$ |
| 6        | $C_2^3$         | $(0, 0)$                   | $U(2)^{\oplus 3} \oplus [-4]^{\oplus 3}$                                                                                                                                                              | —        |
|          |                 | $(96, 0)$                  | $U \oplus U(2)^{\oplus 2} \oplus [-4]^{\oplus 3}$                                                                                                                                                     | $\times$ |
|          |                 | $(112, 0)$                 | $U(2) \oplus [-2]^{\oplus 2} \oplus [-4] \oplus \begin{pmatrix} 0 & 2 \\ 2 & -2 \end{pmatrix}^{\oplus 2}$                                                                                             | —        |
| 7        | $\mathcal{S}_3$ | $(0, 0)$                   | $U \oplus \begin{pmatrix} 2 & -1 & -1 \\ -1 & -4 & -1 \\ -1 & -1 & -4 \end{pmatrix} \oplus \begin{pmatrix} -4 & -2 & 1 & 1 \\ -2 & -4 & -1 & -1 \\ 1 & -1 & -4 & -1 \\ 1 & -1 & -1 & 2 \end{pmatrix}$ | $\times$ |
| 8        | $C_2^2$         | $(48, 0)$                  | $U(2)^{\oplus 3} \oplus [-4]^{\oplus 3}$                                                                                                                                                              | —        |
| 9        | $C_4$           | $(0, 0)$                   | $U(4) \oplus [-2] \oplus [-4] \oplus \begin{pmatrix} 0 & 0 & 0 & 0 & 4 \\ 0 & 0 & 0 & 1 & 1 \\ 0 & 0 & -2 & 0 & 2 \\ 0 & 1 & 0 & 0 & 0 \\ 4 & 1 & 2 & 0 & -2 \end{pmatrix}$                           | $\times$ |
|          |                 | $(104, 0)$                 | $U \oplus U(4) \oplus \begin{pmatrix} 0 & 0 & 0 & 0 & 4 \\ 0 & -2 & 1 & 1 & -2 \\ 0 & 1 & -2 & -1 & -1 \\ 0 & 1 & -1 & -2 & -1 \\ 4 & -2 & -1 & -1 & 2 \end{pmatrix}$                                 | $\times$ |
| 10       | $C_2^4$         | $(0, 0)$                   | $U(2)^{\oplus 3} \oplus [-4] \oplus [-8]$                                                                                                                                                             | —        |
|          |                 | $(160, 0)$                 | $U \oplus U(2)^{\oplus 2} \oplus [-4] \oplus [-8]$                                                                                                                                                    | $\times$ |
| 11       | $C_2^4$         | $(112, 0)$                 | $U(2)^{\oplus 3} \oplus [-4]^{\oplus 2}$                                                                                                                                                              | —        |
| 12       | $C_2^3$         | $(80, 0)$                  | $U(2)^{\oplus 3} \oplus [-4] \oplus [-8]$                                                                                                                                                             | —        |
| 13       | $D_4$           | $(0, 0)$                   | $U \oplus [4]^{\oplus 2} \oplus [-4]^{\oplus 4}$                                                                                                                                                      | $\times$ |

| Leech id | $G$                 | $(\#(-12, 2), \#(-36, 2))$ | $\mathbf{L}_{\mathbf{K3}[3]}^G$                                                                                                                             | $D$      |
|----------|---------------------|----------------------------|-------------------------------------------------------------------------------------------------------------------------------------------------------------|----------|
|          |                     | $(124, 0)$                 | $U \oplus U(4) \oplus [2] \oplus [-2] \oplus [-4]^{\oplus 2}$                                                                                               | $\times$ |
| 14       | #512                | $(256, 0)$                 | $U(2)^{\oplus 3} \oplus [-4]$                                                                                                                               | —        |
| 15       | $\mathcal{A}_{3,3}$ | $(0, 0)$                   | $U(3)^{\oplus 2} \oplus \begin{pmatrix} 2 & -1 & 1 \\ -1 & -4 & -1 \\ 1 & -1 & -4 \end{pmatrix}$                                                            | $\times$ |
| 16       | $C_2^4$             | $(128, 0)$                 | $U(2)^{\oplus 2} \oplus U(4) \oplus [-4]$                                                                                                                   | —        |
|          |                     | $(144, 0)$                 | $U(2)^{\oplus 2} \oplus [-4] \oplus \begin{pmatrix} 0 & 4 \\ 4 & -4 \end{pmatrix}$                                                                          | —        |
| 17       | $\Gamma_{2a_1}$     | $(0, 0)$                   | $U(4) \oplus [-4] \oplus \begin{pmatrix} 0 & 0 & 0 & 4 \\ 0 & 0 & 2 & 2 \\ 0 & 2 & 0 & 0 \\ 4 & 2 & 0 & -4 \end{pmatrix}$                                   | $\times$ |
|          |                     | $(144, 0)$                 | $U \oplus U(4) \oplus [-4] \oplus \begin{pmatrix} 0 & 4 \\ 4 & 4 \end{pmatrix}$                                                                             | $\times$ |
|          |                     | $(128, 0)$                 | $U \oplus U(4)^{\oplus 2} \oplus [-4]$                                                                                                                      | $\times$ |
|          |                     | $(148, 0)$                 | $U(4) \oplus [2] \oplus [-2] \oplus [-4] \oplus \begin{pmatrix} 0 & 2 \\ 2 & 2 \end{pmatrix}$                                                               | —        |
| 18       | $D_6$               | $(0, 0)$                   | $U \oplus U(6) \oplus \begin{pmatrix} 0 & 0 & 6 \\ 0 & -4 & 2 \\ 6 & 2 & -4 \end{pmatrix}$                                                                  | $\times$ |
| 19       | $\mathcal{A}_4$     | $(0, 0)$                   | $U \oplus U(2) \oplus A_2(-4) \oplus [12]$                                                                                                                  | $\times$ |
|          |                     | $(172, 0)$                 | $U^{\oplus 2} \oplus [4] \oplus [-12]^{\oplus 2}$                                                                                                           | $\times$ |
| 20       | $D_5$               | $(0, 0)$                   | $U \oplus \begin{pmatrix} 4 & 1 & 1 & -1 & 1 \\ 1 & 4 & -1 & 1 & -1 \\ 1 & -1 & -6 & -4 & -1 \\ -1 & 1 & -4 & -6 & 1 \\ 1 & -1 & -1 & 1 & -6 \end{pmatrix}$ | $\times$ |
| 21       | $D_4$               | $(72, 0)$                  | $U(2) \oplus [4]^{\oplus 2} \oplus [-4]^{\oplus 3}$                                                                                                         | —        |
| 23       | $C_2^2$             | $(72, 0)$                  | $[2] \oplus [-4]^{\oplus 3} \oplus \begin{pmatrix} 0 & 0 & 4 \\ 0 & 2 & -2 \\ 4 & -2 & -2 \end{pmatrix}$                                                    | $\times$ |

| Leech id | $G$                           | $(\#(-12, 2), \#(-36, 2))$ | $\mathbf{L}_{\mathbf{K3}[3]}^G$                                                                                             | $D$      |
|----------|-------------------------------|----------------------------|-----------------------------------------------------------------------------------------------------------------------------|----------|
| 24       | $C_2^2 \rtimes \mathcal{A}_4$ | $(0, 0)$                   | $U(2) \oplus A_2(2) \oplus [-4] \oplus [-8]$                                                                                | —        |
|          |                               | $(232, 0)$                 | $U \oplus U(2) \oplus [4] \oplus [-24]$                                                                                     | $\times$ |
| 25       | $C_2^5$                       | $(208, 0)$                 | $U(2)^{\oplus 2} \oplus [4] \oplus [-8]$                                                                                    | —        |
|          |                               | $(192, 0)$                 | $U(2)^{\oplus 2} \oplus [4] \oplus [-8]$                                                                                    | —        |
| 26       | $\Gamma_4 a_1$                | $(0, 0)$                   | $U(2) \oplus U(4) \oplus [4] \oplus [-8]$                                                                                   | —        |
|          |                               | $(208, 0)$                 | $U \oplus [4] \oplus [-8] \oplus \begin{pmatrix} 0 & 4 \\ 4 & 4 \end{pmatrix}$                                              | $\times$ |
|          |                               | $(214, 0)$                 | $[2]^{\oplus 2} \oplus [-4] \oplus [-8] \oplus \begin{pmatrix} 0 & 2 \\ 2 & -2 \end{pmatrix}$                               | —        |
| 27       | $C_2 \times \Gamma_2 a_1$     | $(144, 0)$                 | $[4] \oplus [-4] \oplus \begin{pmatrix} 0 & 0 & 0 & 4 \\ 0 & 0 & 2 & -2 \\ 0 & 2 & 0 & -2 \\ 4 & -2 & -2 & 0 \end{pmatrix}$ | —        |
|          |                               | $(168, 0)$                 | $[4] \oplus [-4] \oplus \begin{pmatrix} 0 & 0 & 0 & 4 \\ 0 & 0 & 2 & -2 \\ 0 & 2 & 0 & 0 \\ 4 & -2 & 0 & -4 \end{pmatrix}$  | —        |
| 28       | $2_+^{1+4}$                   | $(0, 0)$                   | $U(4) \oplus \begin{pmatrix} 0 & 4 \\ 4 & 4 \end{pmatrix}^{\oplus 2}$                                                       | —        |
|          |                               | $(172, 0)$                 | $[4]^{\oplus 2} \oplus \begin{pmatrix} 0 & 0 & 0 & 4 \\ 0 & -2 & 2 & 0 \\ 0 & 0 & -2 & -2 \\ 4 & 2 & -2 & 0 \end{pmatrix}$  | —        |
|          |                               | $(168, 0)$                 | $U(2) \oplus U(4)^{\oplus 2}$                                                                                               | $\times$ |
|          |                               | $(168, 16)$                | $U \oplus U(4)^{\oplus 2}$                                                                                                  | —        |
| 29       | $\mathcal{S}_4$               | $(0, 0)$                   | $U \oplus [12]^{\oplus 2} \oplus [-4]^{\oplus 2}$                                                                           | $\times$ |
|          |                               | $(196, 0)$                 | $A_2 \oplus [-4] \oplus [-12] \oplus \begin{pmatrix} 0 & 2 \\ 2 & -2 \end{pmatrix}$                                         | $\times$ |

| Leech id | $G$                           | $(\#(-12, 2), \#(-36, 2))$ | $\mathbf{L}_{\mathbf{K3}[3]}^G$                                                                                             | $D$      |
|----------|-------------------------------|----------------------------|-----------------------------------------------------------------------------------------------------------------------------|----------|
| 30       | $D_4$                         | $(104, 0)$                 | $[2] \oplus [-4] \oplus \begin{pmatrix} 0 & 0 & 0 & 4 \\ 0 & -2 & 0 & -2 \\ 0 & 0 & 8 & -4 \\ 4 & -2 & 2 & 4 \end{pmatrix}$ | $\times$ |
| 31       | $Q_8$                         | $(0, 0)$                   | $[2] \oplus [-4] \oplus \begin{pmatrix} 0 & 0 & 0 & 4 \\ 0 & 4 & 0 & -2 \\ 0 & 0 & -4 & 2 \\ 4 & -2 & 2 & 4 \end{pmatrix}$  | $\times$ |
|          |                               | $(200, 0)$                 | $U \oplus [-2] \oplus \begin{pmatrix} 0 & 0 & 8 \\ 0 & 4 & 4 \\ 8 & 4 & 4 \end{pmatrix}$                                    | $\times$ |
| 32       | $C_2^3$                       | $(84, 0)$                  | $U(4)^{\oplus 2} \oplus \begin{pmatrix} 0 & 4 \\ 4 & 4 \end{pmatrix}$                                                       | —        |
| 33       | #1536                         | $(352, 0)$                 | $U(2) \oplus [12]$                                                                                                          | —        |
| 34       | #1024                         | $(320, 0)$                 | $[4] \oplus \begin{pmatrix} 0 & 0 & 0 & 4 \\ 0 & 0 & 2 & 0 \\ 0 & 2 & 0 & -2 \\ 4 & 0 & -2 & 4 \end{pmatrix}$               | —        |
| 36       | [192, 1541]                   | $(304, 0)$                 | $U(2) \oplus U(4) \oplus [4]$                                                                                               | —        |
|          |                               | $(288, 64)$                | $U(2)^{\oplus 2} \oplus [4]$                                                                                                | —        |
| 37       | $C_4^2 \rtimes \mathcal{A}_4$ | $(0, 0)$                   | $U(2) \oplus [4] \oplus [8] \oplus [-8]$                                                                                    | —        |
|          |                               | $(304, 0)$                 | $U \oplus [4] \oplus [8] \oplus [-8]$                                                                                       | $\times$ |
| 38       | $C_2^2 \rtimes \mathcal{S}_4$ | $(0, 0)$                   | $U(2) \oplus [4] \oplus [12] \oplus [-8]$                                                                                   | —        |
|          |                               | $(256, 0)$                 | $U \oplus [4] \oplus [12] \oplus [-8]$                                                                                      | $\times$ |
|          |                               | $(262, 0)$                 | $[2] \oplus [8] \oplus [-6] \oplus \begin{pmatrix} 0 & 2 \\ 2 & 2 \end{pmatrix}$                                            | —        |
| 39       | $\mathcal{A}_{4,3}$           | $(0, 0)$                   | $[-12] \oplus \begin{pmatrix} 2 & -1 & -1 & -1 \\ -1 & -4 & 2 & 2 \\ -1 & 2 & 4 & 0 \\ -1 & 2 & 0 & 4 \end{pmatrix}$        | $\times$ |

| Leech id | $G$                        | $(\#(-12, 2), \#(-36, 2))$ | $\mathbf{L}_{\mathbf{K3}[3]}^G$                                                                                                          | $D$      |
|----------|----------------------------|----------------------------|------------------------------------------------------------------------------------------------------------------------------------------|----------|
| 40       | $C_2 \times 2_+^{1+4}$     | $(160, 0)$                 | $[4]^{\oplus 2} \oplus [-4] \oplus \begin{pmatrix} 0 & 4 \\ 4 & 4 \end{pmatrix}$                                                         | —        |
|          |                            | $(196, 0)$                 | $U(4) \oplus [4] \oplus \begin{pmatrix} 0 & 4 \\ 4 & 4 \end{pmatrix}$                                                                    | —        |
| 42       | $[64, 202]$                | $(208, 0)$                 | $U(2) \oplus [4]^{\oplus 2} \oplus [-8]$                                                                                                 | —        |
|          |                            | $(232, 0)$                 | $U(2) \oplus [4]^{\oplus 2} \oplus [-8]$                                                                                                 | —        |
| 43       | $\Gamma_{25}a_1$           | $(0, 0)$                   | $U(4) \oplus [8] \oplus \begin{pmatrix} 0 & 4 \\ 4 & 4 \end{pmatrix}$                                                                    | —        |
|          |                            | $(232, 0)$                 | $U(2) \oplus U(4) \oplus [8]$                                                                                                            | $\times$ |
|          |                            | $(236, 0)$                 | $\begin{pmatrix} 0 & 0 & 0 & 0 & 4 \\ 0 & 2 & 0 & 0 & -2 \\ 0 & 0 & 2 & 0 & 2 \\ 0 & 0 & 0 & -8 & 4 \\ 4 & -2 & 2 & 4 & 4 \end{pmatrix}$ | —        |
|          |                            | $(238, 0)$                 | $[2] \oplus [8] \oplus [-2] \oplus \begin{pmatrix} 0 & 4 \\ 4 & 4 \end{pmatrix}$                                                         | —        |
|          |                            | $(232, 32)$                | $U \oplus U(4) \oplus [8]$                                                                                                               | —        |
| 44       | $\mathcal{A}_5$            | $(0, 0)$                   | $U \oplus [60] \oplus \begin{pmatrix} -4 & 2 \\ 2 & 4 \end{pmatrix}$                                                                     | $\times$ |
|          |                            | $(280, 0)$                 | $U \oplus \begin{pmatrix} -4 & -2 & 1 \\ -2 & 4 & -2 \\ 1 & -2 & 16 \end{pmatrix}$                                                       | $\times$ |
| 45       | $C_2 \times \mathcal{S}_4$ | $(0, 0)$                   | $U(2) \oplus [12]^{\oplus 2} \oplus [-4]$                                                                                                | —        |
|          |                            | $(192, 0)$                 | $U \oplus A_2(4) \oplus [-12]$                                                                                                           | $\times$ |
|          |                            | $(220, 0)$                 | $U(2) \oplus [6]^{\oplus 2} \oplus [-4]$                                                                                                 | —        |
| 46       | $[36, 9]$                  | $(0, 0)$                   | $[12] \oplus \begin{pmatrix} -2 & -1 & 0 & -1 \\ -1 & 2 & 1 & 0 \\ 0 & 1 & -2 & -1 \\ -1 & 0 & -1 & 8 \end{pmatrix}$                     | $\times$ |

| Leech id | $G$                          | $(\#(-12, 2), \#(-36, 2))$ | $\mathbf{L}_{\mathbf{K3}[3]}^G$                                                                                    | $D$      |
|----------|------------------------------|----------------------------|--------------------------------------------------------------------------------------------------------------------|----------|
|          |                              | $(272, 0)$                 | $[-12] \oplus \begin{pmatrix} -2 & -1 & 1 & 1 \\ -1 & 2 & 0 & 0 \\ 1 & 0 & 2 & -1 \\ 1 & 0 & -1 & 2 \end{pmatrix}$ | $\times$ |
| 47       | $\mathcal{S}_3^2$            | $(0, 0)$                   | $[12] \oplus \begin{pmatrix} 0 & 0 & 0 & 3 \\ 0 & -4 & -2 & -1 \\ 0 & -2 & 8 & 1 \\ 3 & -1 & 1 & 2 \end{pmatrix}$  | —        |
| 48       | $\Gamma_5 a_2$               | $(168, 0)$                 | $U(4) \oplus [4] \oplus \begin{pmatrix} 0 & 4 \\ 4 & 4 \end{pmatrix}$                                              | $\times$ |
| 49       | $[32, 27]$                   | $(144, 0)$                 | $U(4)^{\oplus 4} \oplus [4]$                                                                                       | —        |
|          |                              | $(180, 0)$                 | $U(4) \oplus [4] \oplus \begin{pmatrix} 0 & 4 \\ 4 & 4 \end{pmatrix}$                                              | —        |
|          |                              | $(168, 32)$                | $[4] \oplus \begin{pmatrix} 0 & 0 & 0 & 4 \\ 0 & 0 & 2 & -2 \\ 0 & 2 & 0 & 0 \\ 4 & -2 & 0 & -4 \end{pmatrix}$     | —        |
| 50       | $C_2^2 \times \mathcal{S}_3$ | $(112, 0)$                 | $U(2) \oplus U(6) \oplus [12]$                                                                                     | —        |
| 51       | $\mathcal{S}_4$              | $(168, 0)$                 | $U(2) \oplus [4]^{\oplus 2} \oplus [-12]$                                                                          | —        |
|          |                              | $(190, 0)$                 | $U(2) \oplus [4]^{\oplus 2} \oplus [-12]$                                                                          | —        |
| 52       | $F_{21}$                     | $(0, 0)$                   | $U \oplus U(7) \oplus [28]$                                                                                        | $\times$ |
| 53       | $F_5$                        | $(0, 0)$                   | $U \oplus [10] \oplus [20] \oplus [-10]$                                                                           | $\times$ |
| 54       | $C_2 \times D_4$             | $(116, 0)$                 | $U(4) \oplus [4] \oplus [8] \oplus [-4]$                                                                           | —        |
| 55       | $QD_{16}$                    | $(0, 0)$                   | $U(8) \oplus [2] \oplus [4] \oplus [-4]$                                                                           | $\times$ |
|          |                              | $(222, 0)$                 | $[2]^{\oplus 2} \oplus \begin{pmatrix} 0 & 0 & 8 \\ 0 & -2 & 4 \\ 8 & 4 & -8 \end{pmatrix}$                        | $\times$ |
|          |                              | $(222, 40)$                | $U \oplus \begin{pmatrix} 0 & 0 & 8 \\ 0 & 2 & 2 \\ 8 & 2 & 2 \end{pmatrix}$                                       | —        |
| 56       | $\mathcal{A}_4$              | $(144, 0)$                 | $U(4)^{\oplus 2} \oplus [4]$                                                                                       | $\times$ |

| Leech id | $G$              | $(\#(-12, 2), \#(-36, 2))$ | $\mathbf{L}_{\mathbf{K3}[3]}^G$                                                                                | $D$      |
|----------|------------------|----------------------------|----------------------------------------------------------------------------------------------------------------|----------|
| 57       | $C_2^3$          | $(108, 16)$                | $[4]^{\oplus 2} \oplus [-4] \oplus \begin{pmatrix} 0 & 4 \\ 4 & 4 \end{pmatrix}$                               | —        |
| 58       | $C_2^3$          | $(146, 0)$                 | $U(4) \oplus [8] \oplus \begin{pmatrix} 0 & 2 \\ 2 & 2 \end{pmatrix}$                                          | —        |
| 59       | $C_2 \times C_4$ | $(172, 0)$                 | $[4] \oplus [8] \oplus \begin{pmatrix} 0 & 0 & 4 \\ 0 & -2 & -2 \\ 4 & -2 & 4 \end{pmatrix}$                   | $\times$ |
|          |                  | $(136, 0)$                 | $[-2] \oplus \begin{pmatrix} 0 & 0 & 0 & 8 \\ 0 & 2 & 0 & -4 \\ 0 & 0 & 4 & 4 \\ 8 & -4 & 4 & 4 \end{pmatrix}$ | $\times$ |
| 60       | $\mathcal{S}_3$  | $(210, 0)$                 | $U(2) \oplus [4] \oplus [6] \oplus [-6]$                                                                       | $\times$ |
| 63       | $C_6$            | $(140, 0)$                 | $U(4) \oplus [4] \oplus \begin{pmatrix} 0 & 4 \\ 4 & 4 \end{pmatrix}$                                          | $\times$ |
| 64       | $C_4$            | $(84, 16)$                 | $U(2) \oplus [4] \oplus [8]$                                                                                   | —        |
| 65       | #6144            | $(448, 0)$                 | $U(2) \oplus [4] \oplus$                                                                                       | —        |
| 66       | #3072            | $(384, 0)$                 | $U(2) \oplus [4] \oplus [12]$                                                                                  | —        |
| 67       | #2048            | $(352, 0)$                 | $[4]^{\oplus 2} \oplus \begin{pmatrix} 0 & 4 \\ 4 & 4 \end{pmatrix}$                                           | —        |
| 69       | $M_{20}$         | $(0, 0)$                   | $[4] \oplus \begin{pmatrix} 4 & 0 & -2 \\ 0 & 4 & -2 \\ -2 & -2 & -8 \end{pmatrix}$                            | —        |
|          |                  | $(400, 0)$                 | $[4] \oplus \begin{pmatrix} -2 & -1 & -1 \\ -1 & 4 & 0 \\ -1 & 0 & 4 \end{pmatrix}$                            | $\times$ |
| 70       | $F_{384}$        | $(0, 0)$                   | $[8]^{\oplus 2} \oplus \begin{pmatrix} 0 & 4 \\ 4 & 4 \end{pmatrix}$                                           | —        |
|          |                  | $(334, 0)$                 | $[8] \oplus \begin{pmatrix} 0 & 0 & 4 \\ 0 & 2 & -2 \\ 4 & -2 & 4 \end{pmatrix}$                               | —        |
|          |                  | $(328, 0)$                 | $U(2) \oplus [8]^{\oplus 2}$                                                                                   | $\times$ |

| Leech id | $G$                 | $(\#(-12, 2), \#(-36, 2))$ | $\mathbf{L}_{K3[3]}^G$                                                                             | $D$      |
|----------|---------------------|----------------------------|----------------------------------------------------------------------------------------------------|----------|
|          |                     | $(328, 48)$                | $U \oplus [8]^{\oplus 2}$                                                                          | —        |
| 71       | [384, 20164]        | $(328, 0)$                 | $[4]^{\oplus 2} \oplus \begin{pmatrix} 0 & 4 \\ 4 & 4 \end{pmatrix}$                               | —        |
|          |                     | $(312, 64)$                | $U(2) \oplus [4]^{\oplus 2}$                                                                       | —        |
| 72       | $\mathcal{A}_6$     | $(0, 0)$                   | $[12] \oplus [-4] \oplus \begin{pmatrix} 2 & 1 \\ 1 & 8 \end{pmatrix}$                             | $\times$ |
|          |                     | $(380, 0)$                 | $A_2 \oplus [2] \oplus [-30]$                                                                      | $\times$ |
| 73       | $\mathcal{A}_{4,4}$ | $(0, 0)$                   | $A_2(2) \oplus 4 \oplus [-24]$                                                                     | —        |
|          |                     | $(304, 0)$                 | $[-24] \oplus \begin{pmatrix} 2 & 0 & 1 \\ 0 & 2 & -1 \\ 1 & -1 & 4 \end{pmatrix}$                 | $\times$ |
| 74       | $H_{192}$           | $(0, 0)$                   | $[8] \oplus [12] \oplus \begin{pmatrix} 0 & 4 \\ 4 & 4 \end{pmatrix}$                              | —        |
|          |                     | $(286, 0)$                 | $[2]^{\oplus 2} \oplus [12] \oplus [-8]$                                                           | —        |
| 75       | [192, 1538]         | $(280, 0)$                 | $[4] \oplus \begin{pmatrix} 4 & 0 & 2 \\ 0 & 4 & -2 \\ 2 & -2 & -4 \end{pmatrix}$                  | —        |
|          |                     | $(240, 0)$                 | $U(2) \oplus [8] \oplus [12]$                                                                      | —        |
| 76       | $T_{192}$           | $(0, 0)$                   | $A_2(4) \oplus [4] \oplus [-4]$                                                                    | —        |
|          |                     | $(370, 0)$                 | $\begin{pmatrix} 0 & 0 & 0 & 4 \\ 0 & 2 & 0 & -2 \\ 0 & 0 & 6 & 2 \\ 4 & -2 & 2 & 4 \end{pmatrix}$ | —        |
|          |                     | $(360, 0)$                 | $U(2) \oplus A_2(4)$                                                                               | $\times$ |
|          |                     | $(360, 64)$                | $U \oplus A_2(4)$                                                                                  | —        |
| 77       | $L_2(7)$            | $(0, 0)$                   | $[28] \oplus [-4] \oplus \begin{pmatrix} 2 & 1 \\ 1 & 4 \end{pmatrix}$                             | $\times$ |
|          |                     | $(364, 0)$                 | $U \oplus [14]^{\oplus 2}$                                                                         | $\times$ |
| 79       | [128, 1758]         | $(192, 0)$                 | $U(4) \oplus [4] \oplus [8]$                                                                       | —        |
|          |                     | $(262, 0)$                 | $[4] \oplus [8] \oplus \begin{pmatrix} 0 & 4 \\ 4 & 4 \end{pmatrix}$                               | —        |



| Leech id | $G$                          | $(\#(-12, 2), \#(-36, 2))$ | $\mathbf{L}_{\mathbf{K3}[3]}^G$                                                                  | $D$      |
|----------|------------------------------|----------------------------|--------------------------------------------------------------------------------------------------|----------|
| 81       | [128, 1755]                  | (224, 0)                   | $U(4) \oplus [4] \oplus [8]$                                                                     | —        |
|          |                              | (260, 0)                   | $U(4) \oplus [4] \oplus [8]$                                                                     | —        |
| 82       | $\mathcal{S}_5$              | (0, 0)                     | $U \oplus [20] \oplus [60]$                                                                      | $\times$ |
| 83       | $C_2^2 \times \mathcal{S}_4$ | (208, 0)                   | $U(2) \oplus [12]^{\oplus 2}$                                                                    | —        |
| 84       | $M_9$                        | (0, 0)                     | $[4] \oplus [-6] \oplus \begin{pmatrix} 4 & 2 \\ 2 & 10 \end{pmatrix}$                           | $\times$ |
|          |                              | (344, 0)                   | $[12] \oplus \begin{pmatrix} -2 & -1 & 0 \\ -1 & 2 & -1 \\ 0 & -1 & 4 \end{pmatrix}$             | $\times$ |
| 85       | $N_{72}$                     | (0, 0)                     | $[12]^{\oplus 2} \oplus \begin{pmatrix} 0 & 3 \\ 3 & 2 \end{pmatrix}$                            | —        |
| 86       | $D_4^2$                      | (188, 32)                  | $U(4) \oplus [4]^{\oplus 2}$                                                                     | —        |
| 87       | $T_{48}$                     | (0, 0)                     | $A_2(8) \oplus [2] \oplus [-4]$                                                                  | $\times$ |
| 88       | $C_2 \times \mathcal{S}_4$   | (180, 0)                   | $[4]^{\oplus 3} \oplus [-12]$                                                                    | —        |
| 89       | [32, 43]                     | (208, 0)                   | $U(8) \oplus [2] \oplus [4]$                                                                     | $\times$ |
|          |                              | (244, 0)                   | $U(8) \oplus [2] \oplus [4]$                                                                     | $\times$ |
| 90       | $\mathcal{S}_4$              | (188, 0)                   | $A_2(2) \oplus [4] \oplus [-24]$                                                                 | —        |
| 91       | $\mathcal{S}_4$              | (156, 24)                  | $U(4) \oplus [4]^{\oplus 2}$                                                                     | —        |
| 92       | $\mathcal{S}_4$              | (270, 0)                   | $[2] \oplus [4] \oplus [6] \oplus [-8]$                                                          | $\times$ |
| 94       | $C_2 \times Q_8$             | (316, 0)                   | $[2]^{\oplus 2} \oplus [4] \oplus [-16]$                                                         | $\times$ |
| 95       | $C_2 \times D_4$             | (196, 8)                   | $[8]^{\oplus 2} \oplus \begin{pmatrix} 0 & 2 \\ 2 & 2 \end{pmatrix}$                             | —        |
| 97       | $D_6$                        | (230, 0)                   | $\begin{pmatrix} 0 & 0 & 0 & 6 \\ 0 & 4 & 0 & 2 \\ 0 & 0 & 4 & 2 \\ 6 & 2 & 2 & 2 \end{pmatrix}$ | $\times$ |
| 99       | #245760                      | (640, 0)                   | $[4]^{\oplus 3}$                                                                                 | —        |
| 100      | #30720                       | (576, 0)                   | $\begin{pmatrix} 4 & -2 & 2 \\ -2 & 4 & -2 \\ 2 & -2 & 8 \end{pmatrix}$                          | —        |

| Leech id | $G$                 | $(\#(-12, 2), \#(-36, 2))$ | $\mathbf{L}_{\mathbf{K3}[3]}^G$                                           | $D$      |
|----------|---------------------|----------------------------|---------------------------------------------------------------------------|----------|
| 102      | $L_3(4)$            | $(0, 0)$                   | $[12] \oplus \begin{pmatrix} 4 & 2 \\ 2 & 8 \end{pmatrix}$                | —        |
|          |                     | $(0, 0)$                   | $A_2(2) \oplus [28]$                                                      | —        |
|          |                     | $(560, 0)$                 | $[12] \oplus \begin{pmatrix} 2 & 1 \\ 1 & 4 \end{pmatrix}$                | —        |
|          |                     | $(560, 0)$                 | $\begin{pmatrix} 4 & 2 & 1 \\ 2 & 4 & -1 \\ 1 & -1 & 8 \end{pmatrix}$     | $\times$ |
| 103      | #12288              | $(480, 0)$                 | $[4]^{\oplus 2} \oplus [8]$                                               | —        |
| 104      | #9216               | $(448, 0)$                 | $A_2(2) \oplus [12]$                                                      | —        |
| 105      | #6144               | $(416, 0)$                 | $[4]^{\oplus 2} \oplus [12]$                                              | —        |
| 106      | $C_2^4 \rtimes A_6$ | $(0, 0)$                   | $[4]^{\oplus 2} \oplus [24]$                                              | —        |
|          |                     | $(520, 0)$                 | $\begin{pmatrix} 4 & 0 & -2 \\ 0 & 4 & -2 \\ -2 & -2 & 8 \end{pmatrix}$   | $\times$ |
|          |                     | $(530, 0)$                 | $[2]^{\oplus 2} \oplus [24]$                                              | —        |
|          |                     | $(520, 80)$                | $\begin{pmatrix} 2 & 1 & 1 \\ 1 & 4 & 0 \\ 1 & 0 & 4 \end{pmatrix}$       | —        |
| 108      | $\mathcal{A}_7$     | $(0, 0)$                   | $\begin{pmatrix} 4 & 0 & -2 \\ 0 & 6 & -3 \\ -2 & -3 & 20 \end{pmatrix}$  | $\times$ |
|          |                     | $(0, 0)$                   | $\begin{pmatrix} 4 & -1 & 1 \\ -1 & 8 & 1 \\ 1 & 1 & 14 \end{pmatrix}$    | —        |
|          |                     | $(0, 0)$                   | $\begin{pmatrix} 2 & -1 & 1 \\ -1 & 16 & -6 \\ 1 & -6 & 16 \end{pmatrix}$ | —        |
| 110      | [1920, 240993]      | $(0, 0)$                   | $[4]^{\oplus 2} \oplus [40]$                                              | —        |
|          |                     | $(0, 0)$                   | $[8] \oplus \begin{pmatrix} 8 & 4 \\ 4 & 12 \end{pmatrix}$                | —        |

| Leech id | $G$             | $(\#(-12, 2), \#(-36, 2))$ | $\mathbf{L}_{\mathbf{K3}[3]}^G$                                          | $D$      |
|----------|-----------------|----------------------------|--------------------------------------------------------------------------|----------|
|          |                 | $(0, 0)$                   | $[8] \oplus \begin{pmatrix} 8 & 4 \\ 4 & 12 \end{pmatrix}$               | —        |
|          |                 | $(430, 0)$                 | $[2] \oplus [8] \oplus [10]$                                             | —        |
|          |                 | $(430, 0)$                 | $[2]^{\oplus 2} \oplus [40]$                                             | —        |
| 111      | [1344, 11686]   | $(0, 0)$                   | $\begin{pmatrix} 8 & -4 & 4 \\ -4 & 8 & -4 \\ 4 & -4 & 12 \end{pmatrix}$ | —        |
|          |                 | $(490, 0)$                 | $[2] \oplus \begin{pmatrix} 6 & -2 \\ -2 & 10 \end{pmatrix}$             | —        |
| 112      | [1152, 155478]  | $(0, 0)$                   | $[8]^{\oplus 2} \oplus [12]$                                             | —        |
| 113      | [1152, 157862]  | $(376, 0)$                 | $[4]^{\oplus 2} \oplus [12]$                                             | —        |
|          |                 | $(360, 64)$                | $A_2(2) \oplus [4]$                                                      | —        |
| 115      | [768, 1090134]  | $(288, 0)$                 | $[4] \oplus [8]^{\oplus 2}$                                              | —        |
|          |                 | $(358, 0)$                 | $[4] \oplus [8]^{\oplus 2}$                                              | —        |
| 117      | [768, 1090070]  | $(336, 64)$                | $[4]^{\oplus 3}$                                                         | —        |
| 118      | $\mathcal{S}_6$ | $(0, 0)$                   | $[12] \oplus \begin{pmatrix} 8 & -2 \\ -2 & 8 \end{pmatrix}$             | —        |
|          |                 | $(0, 0)$                   | $[12] \oplus \begin{pmatrix} 8 & -2 \\ -2 & 8 \end{pmatrix}$             | —        |
|          |                 | $(360, 0)$                 | $[12] \oplus \begin{pmatrix} 2 & -1 \\ -1 & 8 \end{pmatrix}$             | —        |
|          |                 | $(360, 0)$                 | $\begin{pmatrix} 6 & 0 & -3 \\ 0 & 6 & -3 \\ -3 & -3 & 8 \end{pmatrix}$  | —        |
| 119      | $M_{10}$        | $(0, 0)$                   | $[4]^{\oplus 2} \oplus [30]$                                             | $\times$ |
|          |                 | $(0, 0)$                   | $[2] \oplus [12] \oplus [20]$                                            | —        |
|          |                 | $(0, 0)$                   | $[2] \oplus [12] \oplus [20]$                                            | —        |
|          |                 | $(470, 0)$                 | $A_2(2) \oplus [2]$                                                      | —        |
|          |                 | $(470, 0)$                 | $[2]^{\oplus 2} \oplus [30]$                                             | $\times$ |
|          |                 | $(470, 72)$                | $[2] \oplus \begin{pmatrix} 2 & -1 \\ -1 & 8 \end{pmatrix}$              | —        |

| Leech id | $G$                          | $(\#(-12, 2), \#(-36, 2))$ | $\mathbf{L}_{\mathbf{K3}[3]}^G$                                        | $D$      |
|----------|------------------------------|----------------------------|------------------------------------------------------------------------|----------|
| 120      | $L_2(11)$                    | $(0, 0)$                   | $\begin{pmatrix} 4 & 2 & 2 \\ 2 & 12 & 1 \\ 2 & 1 & 12 \end{pmatrix}$  | $\times$ |
|          |                              | $(0, 0)$                   | $\begin{pmatrix} 4 & 2 & 1 \\ 2 & 12 & 6 \\ 1 & 6 & 14 \end{pmatrix}$  | —        |
| 121      | $[576, 8654]$                | $(0, 0)$                   | $[8] \oplus [12]^{\oplus 2}$                                           | —        |
|          |                              | $(0, 0)$                   | $[8] \oplus [12]^{\oplus 2}$                                           | —        |
|          |                              | $(334, 0)$                 | $[6]^{\oplus 2} \oplus [8]$                                            | —        |
| 122      | $[500, 23]$                  | $(0, 0)$                   | $A_3(5)$                                                               | —        |
| 124      | $[384, 18134]$               | $(456, 0)$                 | $[2] \oplus [4] \oplus [16]$                                           | $\times$ |
| 125      | $[384, 17948]$               | $(256, 0)$                 | $[4] \oplus [8] \oplus [12]$                                           | —        |
|          |                              | $(256, 0)$                 | $[4] \oplus [8] \oplus [12]$                                           | —        |
| 126      | $[384, 20089]$               | $(352, 0)$                 | $A_2(4) \oplus [4]$                                                    | —        |
|          |                              | $(388, 0)$                 | $A_2(4) \oplus [4]$                                                    | —        |
| 127      | $\mathcal{A}_6$              | $(430, 0)$                 | $A_2(2) \oplus [12]$                                                   | —        |
| 128      | $\Gamma L_2(\mathbb{F}_4)$   | $(0, 0)$                   | $\begin{pmatrix} 8 & 2 & -3 \\ 2 & 8 & 3 \\ -3 & 3 & 18 \end{pmatrix}$ | —        |
|          |                              | $(0, 0)$                   | $[60] \oplus \begin{pmatrix} 2 & 1 \\ 1 & 8 \end{pmatrix}$             | —        |
| 129      | $C_2 \times L_2(7)$          | $(0, 0)$                   | $[28] \oplus \begin{pmatrix} 4 & 2 \\ 2 & 8 \end{pmatrix}$             | —        |
|          |                              | $(0, 0)$                   | $[28] \oplus \begin{pmatrix} 4 & 2 \\ 2 & 8 \end{pmatrix}$             | —        |
| 131      | $[192, 1494]$                | $(312, 0)$                 | $[4] \oplus [8]^{\oplus 2}$                                            | $\times$ |
| 132      | $T_{192}$                    | $(312, 48)$                | $[4]^{\oplus 3}$                                                       | —        |
| 133      | $C_2 \times M_9$             | $(428, 0)$                 | $[2]^{\oplus 2} \oplus [36]$                                           | —        |
|          |                              | $(428, 0)$                 | $[4] \oplus \begin{pmatrix} 4 & -2 \\ -2 & 10 \end{pmatrix}$           | $\times$ |
| 134      | $\text{AGL}_1(\mathbb{F}_9)$ | $(0, 0)$                   | $[2] \oplus [12] \oplus [36]$                                          | —        |

| Leech id | $G$                                  | $(\#(-12, 2), \#(-36, 2))$ | $\mathbf{L}_{\mathbf{K3}[3]}^G$                                       | $D$      |
|----------|--------------------------------------|----------------------------|-----------------------------------------------------------------------|----------|
|          |                                      | $(0, 0)$                   | $[2] \oplus [12] \oplus [36]$                                         | —        |
| 135      | $\mathcal{S}_3 \times \mathcal{S}_4$ | $(204, 0)$                 | $A_2(4) \oplus [12]$                                                  | —        |
|          |                                      | $(204, 0)$                 | $A_2(4) \oplus [12]$                                                  | —        |
| 136      | $\mathcal{S}_5$                      | $(298, 0)$                 | $\begin{pmatrix} 8 & 2 & -2 \\ 2 & 8 & 2 \\ -2 & 2 & 8 \end{pmatrix}$ | —        |
| 137      | $\mathcal{S}_5$                      | $(350, 0)$                 | $[4] \oplus [6] \oplus [10]$                                          | $\times$ |
|          |                                      | $(350, 0)$                 | $[2]^{\oplus 2} \oplus [60]$                                          | —        |
| 139      | $[96, 195]$                          | $(252, 0)$                 | $[4] \oplus [12]^{\oplus 2}$                                          | —        |
| 143      | $[64, 257]$                          | $(270, 16)$                | $\begin{pmatrix} 6 & 2 & -2 \\ 2 & 6 & 2 \\ -2 & 2 & 6 \end{pmatrix}$ | —        |
| 146      | $C_2 \times \mathcal{S}_4$           | $(290, 0)$                 | $[4]^{\oplus 2} \oplus [24]$                                          | —        |
| 148      | $C_2 \times \mathcal{S}_4$           | $(296, 24)$                | $[2] \oplus [6] \oplus [8]$                                           | —        |
| 149      | $C_2 \times F_5$                     | $(232, 0)$                 | $[20] \oplus \begin{pmatrix} 4 & 2 \\ 2 & 6 \end{pmatrix}$            | —        |
|          |                                      | $(232, 0)$                 | $[4] \oplus [10]^{\oplus 2}$                                          | $\times$ |
| 152      | $C_2 \times QD_{16}$                 | $(340, 40)$                | $[2] \oplus \begin{pmatrix} 6 & -2 \\ -2 & 6 \end{pmatrix}$           | —        |
| 160      | $C_2^2 \rtimes C_4$                  | $(174, 24)$                | $[4] \oplus [8]^{\oplus 2}$                                           | —        |

Table 2: Symplectic birational groups with trivial discriminant action
